# Supplementary material for: UrbanGS: Semantic-Guided Gaussian Splatting for Urban Scene Reconstruction
Source: arXiv:2412.03473 source file (2025-03-21)
Supplement: Supplementary file 1 [file X_suppl.tex]

% \clearpage
\setcounter{page}{1}
% \maketitlesupplementary

% \begin{figure*}[!ht]
%     \centering
%     \includegraphics[width=\textwidth]{figure/suppliment.pdf}
%     \caption{Qualitative comparison on the PandaSet~\cite{xiao2021pandaset} dataset. We demonstrate the qualitative comparison results with our main competitors PVG~\cite{chen2023periodic} and 3DGS~\cite{kerbl20233d} on driving scenes reconstruction of PandaSet~\cite{xiao2021pandaset}. Our method achieves better visual quality for both static and dynamic objects, showing clearer details and more accurate motion handling. From left to right: ground truth image, PVG~\cite{chen2023periodic} results, 3DGS~\cite{kerbl20233d} results, and our results.}
%     \label{s}
% \end{figure*}

% \begin{figure*}[htb]
% \begin{minipage}[b]{1.0\linewidth}
%   \centering
%   \centerline{\includegraphics[width=18cm]{figure/suppliment.pdf}}
% \end{minipage}
% \caption{Visual comparison of different methods. (a) LDCT denoising. (The display window is [-160, 240] HU.) (b) MRI super-resolution. (c) MRI artifact removal. Zoomed ROI of the rectangle region is recommended for better visualization. Yellow arrows in (a) indicate regions with notable differences.}
% \label{visual compare}
% \end{figure*}

\section{Network Architecture Details}

Our deformation MLP adopts a simple yet effective architecture with 3 hidden layers, each having a width of 64 neurons. The network takes time embeddings, timestamps and positions as input and processes them through a sequence of linear layers followed by ReLU activation functions. For timestamp input $t$, we first lift it to a higher dimensional space through positional encoding:
\begin{equation}
    \gamma(t) = (\sin(2^0\pi t), \cos(2^0\pi t), \dots, 
\end{equation}
\begin{equation}
    \sin(2^{L-1}\pi t), \cos(2^{L-1}\pi t))
\end{equation}
where $L=8$ is the number of frequency bands. The embedded features are then processed through the network:
\begin{equation}
    \begin{split}
    \text{Input} & \rightarrow \text{Linear}(64) \rightarrow \text{ReLU} \\
    & \rightarrow \text{Linear}(64) \rightarrow \text{ReLU} \\
    & \rightarrow \text{Linear}(64) \rightarrow \text{ReLU}
    \end{split}
\end{equation}
The output features from the final ReLU layer are then processed by four parallel linear layers to predict different residuals. This design allows the network to learn specialized representations for different deformation parameters while sharing common temporal feature extraction in the backbone layers.

\section{Ablation Study on Time Embedding}

We conducted extensive experiments on different dimensions of time embedding using the PandaSet~\cite{xiao2021pandaset} dataset to investigate its impact on reconstruction quality. Table~\ref{tab:time_embedding} shows the quantitative comparison of varying embedding dimensions from 4 to 32:

\begin{table}[h]
\centering
\caption{Quantitative results with different time embedding dimensions on PandaSet~\cite{xiao2021pandaset}}
\label{tab:time_embedding}
\begin{tabular}{cccc}
\hline
Dimension & PSNR↑ & SSIM↑ \\
\hline
4  & 26.45 & 0.812 \\
8  & 26.56 & 0.814 \\
16 & 26.53 & \textbf{0.816} \\
32 & \textbf{26.58} & 0.814 \\
\hline
\end{tabular}
\end{table}

As shown in the results, increasing the embedding dimension beyond 8 only brings marginal improvements (less than 0.1 dB in PSNR). Considering the trade-off between performance and computational efficiency, we choose 8-dimensional time embedding as our default setting, which achieves a good balance between reconstruction quality and training speed.

\section{Visualization on PandaSet}

We provide extensive qualitative comparisons with PVG~\cite{chen2023periodic} and 3DGS~\cite{kerbl20233d} on the PandaSet~\cite{xiao2021pandaset} dataset. As shown in Figure~\ref{fig:sub}, our method achieves superior visual quality for both static and dynamic objects.

\section{Limitations}

While our method achieves superior visual quality, it comes with increased computational overhead. The main bottleneck is that our approach requires MLP inference for potential dynamic Gaussian points to extract transformation attributes. This leads to slower rendering speed compared to some existing methods. Table 2 shows the rendering efficiency comparison, all measured on a single NVIDIA V100S GPU with the image resolution of 1920×1080:

\begin{table}[h]
\centering
\caption{Rendering speed comparison on PandaSet~\cite{xiao2021pandaset}}
\begin{tabular}{cc}
\hline
Method & Rendering Speed (FPS) \\
\hline
EmerNeRF~\cite{yang2023emernerf} & 0.03 \\
Ours & 15.9 \\
PVG~\cite{chen2023periodic} & 25.6 \\
3DGS~\cite{kerbl20233d} & \textbf{30.4} \\
\hline
\end{tabular}
\end{table}

Although our method is significantly faster than NeRF-based approaches, it runs approximately 1.6× slower than PVG and 1.9× slower than 3DGS during rendering. Future work will focus on addressing these computational efficiency challenges and improving scene reconstruction quality through techniques like more efficient dynamic point handling strategies.
